# Supplementary material for: StrataFlux: Memory-Hierarchy-Native Low-Bit LLM Inference
Source: arXiv:2611.08363 source file (2026-11-05)
Supplement: Supplementary file 1 [file appendix_setup.tex]

\makeatletter
\long\def\LT@makecaption#1#2#3{%
  \LT@mcol\LT@cols c{\hbox to\z@{\hss\parbox[t]{\textwidth}{\@makecaption{#2}{#3}\vskip\baselineskip}\hss}}}
\makeatother
% Use the conference template's default figure-to-text spacing.
\definecolor{codeframe}{rgb}{0.75,0.75,0.75}
\definecolor{codebackground}{rgb}{0.97,0.97,0.97}
\mlsystitlerunning{\paperrunningtitle}

% Measure each column table before placing it, so it cannot run past a column.
\newsavebox{\appendixcolumnbox}
\newdimen\appendixcolumnheight
\NewDocumentEnvironment{appendixcolumntable}{+b}{%
\par\setbox\appendixcolumnbox=\vbox{\hsize=\linewidth\begin{table}[H]#1\end{table}}%
\penalty0\box\appendixcolumnbox\par\penalty0
}{}

\makeatletter
\newcommand{\appendixgroupreserve}[1]{%
\noalign{\global\let\ST@next\@empty
\global\@tempdima=#1\ST@rowht\global\advance\@tempdima 2\ST@rowht}%
\ifdim\ST@pageleft<\@tempdima\ST@newpage\fi\ST@next
}
\newcommand{\appendixfirstgroupreserve}[1]{%
\par\penalty0\begingroup
\dimen@=#1\normalbaselineskip\advance\dimen@ 6\normalbaselineskip
\@tempdima=\pagegoal\advance\@tempdima-\pagetotal
\ifdim\@tempdima<\dimen@\newpage\fi
\endgroup
}
\newenvironment{appendixflowtable}{\par\appendixfirstgroupreserve{5}\begingroup\def\@captype{table}\centering}{\par\endgroup\medskip}
\makeatother
\newcommand{\appendixwideinput}[1]{\input{#1}}
\newcommand{\appendixgroup}[1]{%
\par\medskip\noindent\textbf{#1}\par\nopagebreak
\vspace{2pt}\hrule height 0.3pt\nobreak\vspace{4pt}\ignorespaces
}
\newcommand{\additionalweightstable}[1]{%
\begingroup\setlength{\tabcolsep}{3pt}\renewcommand{\arraystretch}{1.08}\fontsize{8}{9.5}\selectfont
\def\appendixmatrixcaption{}
\input{tables/generated/appendix_completion_weights_matrix_#1}
\endgroup
}
\newcommand{\additionalkvtable}[1]{%
\begingroup\setlength{\tabcolsep}{3pt}\renewcommand{\arraystretch}{1.08}\fontsize{8}{9.5}\selectfont
\def\appendixmatrixcaption{}
\input{tables/generated/appendix_completion_kv_matrix_#1}
\endgroup
}
\newcommand{\additionaljointtable}[1]{%
\begingroup\setlength{\tabcolsep}{3pt}\renewcommand{\arraystretch}{1.08}\fontsize{8}{9.5}\selectfont
\def\appendixmatrixcaption{}
\input{tables/generated/appendix_completion_joint_matrix_#1}
\endgroup
}
